# Supplementary material for: Local density approximations from finite systems
Source: arXiv:1611.01443 ancillary file (2016-11-29)
Supplement: Supplementary file 1 [file Supplemental_Material.pdf]

# Local density approximations from finite systems (supplemental material)

M. T. Entwistle
*Department of Physics, University of York, and European Theoretical Spectroscopy Facility, Heslington, York YO10 5DD, United Kingdom and Fitzwilliam College, University of Cambridge, Cambridge CB3 0DG, United Kingdom*

M. J. P. Hodgson, J. Wetherell, B. Longstaff,* J. D. Ramsden, and R. W. Godby
*Department of Physics, University of York, and European Theoretical Spectroscopy Facility, Heslington, York YO10 5DD, United Kingdom*

(Dated: November 29, 2016)

## INITIAL LDAS

The initial LDAs are (we use Hartree atomic units):

$$1e : \varepsilon_{\text{xc}}(n) = (-(0.775 \pm 0.005) + (0.77 \pm 0.02)n - (0.44 \pm 0.01)n^2)n^{(0.638 \pm 0.002)} \tag{1}$$

$$2e : \varepsilon_{\text{xc}}(n) = (-(0.71 \pm 0.01) + (0.63 \pm 0.04)n - (0.34 \pm 0.03)n^2)n^{(0.604 \pm 0.006)} \tag{2}$$

$$3e : \varepsilon_{\text{xc}}(n) = (-(0.74 \pm 0.02) + (0.74 \pm 0.05)n - (0.44 \pm 0.04)n^2)n^{(0.61 \pm 0.01)}. \tag{3}$$

## REFINED LDAS

The refined LDAs are:

$$\begin{aligned} 1e : \varepsilon_{\text{xc}}(n) &= (-(0.803 \pm 0.003) + (0.82 \pm 0.01)n - (0.47 \pm 0.01)n^2)n^{(0.638 \pm 0.001)} \\ V_{\text{xc}}(n) &= (-(1.315 \pm 0.004) + (2.16 \pm 0.02)n - (1.71 \pm 0.03)n^2)n^{(0.638 \pm 0.001)} \end{aligned} \tag{4}$$

$$\begin{aligned} 2e : \varepsilon_{\text{xc}}(n) &= (-(0.74 \pm 0.01) + (0.68 \pm 0.04)n - (0.38 \pm 0.03)n^2)n^{(0.604 \pm 0.006)} \\ V_{\text{xc}}(n) &= (-(1.19 \pm 0.01) + (1.77 \pm 0.08)n - (1.37 \pm 0.09)n^2)n^{(0.604 \pm 0.006)} \end{aligned} \tag{5}$$

$$\begin{aligned} 3e : \varepsilon_{\text{xc}}(n) &= (-(0.77 \pm 0.02) + (0.79 \pm 0.05)n - (0.48 \pm 0.04)n^2)n^{(0.61 \pm 0.01)} \\ V_{\text{xc}}(n) &= (-(1.24 \pm 0.02) + (2.1 \pm 0.1)n - (1.7 \pm 0.1)n^2)n^{(0.61 \pm 0.01)}. \end{aligned} \tag{6}$$

## SYSTEM 1 (TWO-ELECTRON TRIPLE WELL)

The external potential is:

$$V_{\text{ext}} = -\frac{3}{5}e^{-\frac{1}{4}(x+5)^2} - 2e^{-\frac{2}{5}x^2} - \frac{3}{5}e^{-\frac{1}{4}(x-5)^2} + \frac{1}{2}. \tag{7}$$

For this system converged results are obtained with a spatial grid spacing $\delta x = 0.05$ a.u. Fig. 1 shows the external potential and the exact ground-state electron density.

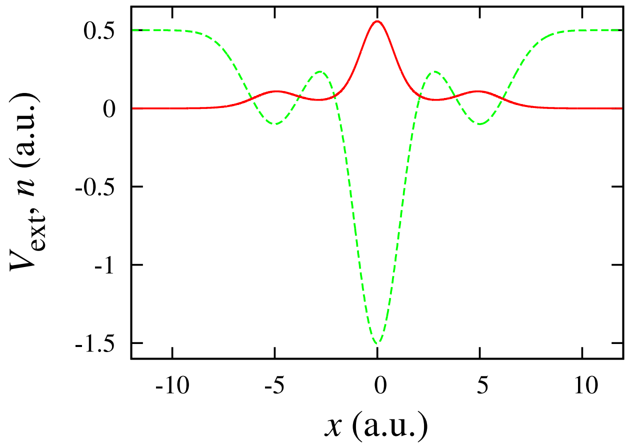


FIG. 1: System 1 (two-electron triple well). The external potential (dashed green line) and the exact ground-state electron density (solid red line).

## SYSTEM 2 (ONE-ELECTRON HARMONIC WELL)

The external potential is:

$$V_{\text{ext}} = \frac{1}{2}\omega^2 x^2, \tag{8}$$

where $\omega = \frac{51}{200}$ a.u., with $\delta x = 0.05$ a.u. Fig. 2 shows the external potential and the exact ground-state electron density.

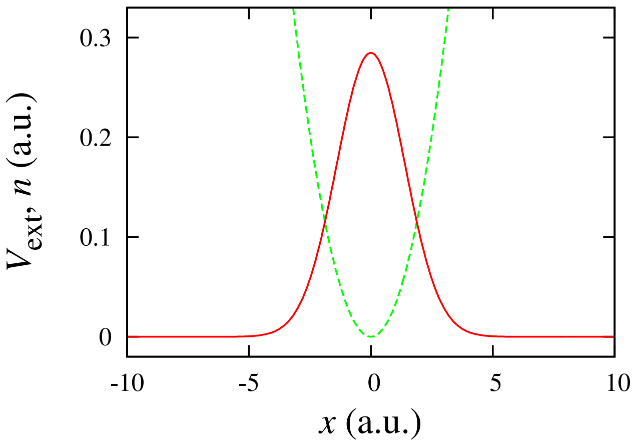


FIG. 2: System 2 (one-electron harmonic well). The external potential (dashed green line) and the exact ground-state electron density (solid red line).

## SYSTEMS 3A AND 3B (TWO-ELECTRON HARMONIC WELLS)

### A. Strongly-confined harmonic well

The external potential is:

$$V_{\text{ext}} = \frac{1}{2}\omega^2 x^2, \tag{9}$$

where $\omega = \frac{2}{5}$ a.u., with $\delta x = 0.05$ a.u. Fig. 3(a) shows the external potential and the exact ground-state electron density.

### B. Weakly-confined harmonic well

The external potential is:

$$V_{\mathrm{ext}} = \frac{1}{2}\omega^2 x^2, \tag{10}$$

where $\omega = \frac{1}{100}$ a.u., with $\delta x = 0.13$ a.u. Fig. 3(b) shows the external potential and the exact ground-state electron density.

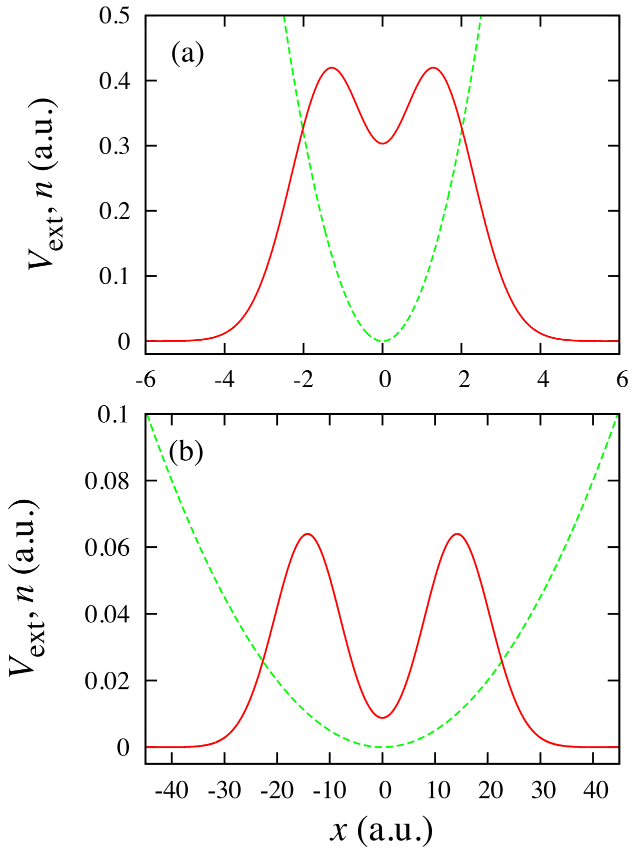


FIG. 3: Two-electron harmonic wells. (a) System 3A (strongly-confined harmonic well). The external potential (dashed green line) and the exact ground-state electron density (solid red line). (b) System 3B (weakly-confined harmonic well). The external potential (dashed green line) and the exact ground-state electron density (solid red line).

## SYSTEM 4 (TUNNELING SYSTEM)

The ground-state external potential is:

$$V_{\mathrm{ext}} = \alpha x^{10} - \beta x^4, \tag{11}$$

where $\alpha = 5 \times 10^{-11}$ a.u. and $\beta = 5 \times 10^{-5}$ a.u., with $\delta x = 0.1$ a.u. and a temporal grid spacing $\delta t = 1 \times 10^{-3}$ a.u. For $t > 0$ a perturbing electric field ($V_{\mathrm{pert}} = -0.01x$) is applied to induce quantum tunneling. Fig. 4 (a) shows the ground-state external potential and the time-dependent external potential. Fig. 4 (b) shows the exact ground-state electron density and the exact electron density at $t = 40$ a.u.

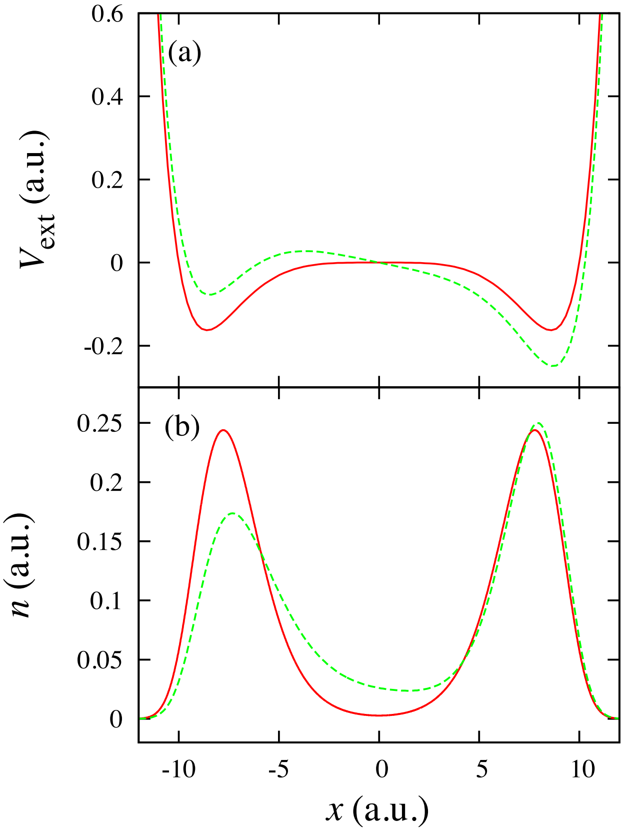


FIG. 4: System 4 (tunneling system). (a) The ground-state external potential (solid red line) and the time-dependent external potential (dashed green line). (b) The exact ground-state electron density (solid red line) and the exact electron density at $t = 40$ a.u. (dashed green line).

---

* Present Address: Department of Mathematics, Imperial College London, London SW7 2AZ, United Kingdom
